# Supplementary material for: Distributionally Robust Kalman Filtering over Finite and Infinite Horizon
Source: arXiv:2407.18837 source file (2024-07-26)
Supplement: Supplementary file 1 [file appendix_optimality_results.tex]

For a fixed $\gamma > {\gamma}_{\RO}$, utilizing an optimization oracle to solve \cref{eq:infinite DRRO reformulation} for $\K$ and obtain a $\gamma$-optimal controller, denoted as $\K_{\gamma,\star}$, enables us to find the optimal \DRO~controller by determining the optimal $\gamma_\star$ through \cref{eq:worst_gamma}. Our attention thus shifts to the $\gamma$-optimal problem detailed below.

This section introduces the primary theoretical findings. In particular, \cref{thm:infinite strong duality} establishes the strong duality of the infinite-horizon worst-case expected regret, denoted as $R(\K,r)$ and introduced in \cref{def:worst case regret}. The strong duality outlined in \cref{thm:infinite strong duality} offers a pathway to determine the optimal \DRO~controller by finding the saddle point of a min-max problem in \cref{thm:kkt}. Furthermore, \cref{thm:kkt} presents the necessary and sufficient optimality conditions for the saddle point solution of the min-max problem. Via this result, \cref{thm:convergence of the costs} concludes that the time-averaged optimum worst-case expected regret of the finite-horizon and infinite-horizon problems coincide as $T\to\infty$.

\subsection{Reduction to a Suboptimal Problem via Strong Duality}

\citet{DRORO} shows that the finite-horizon worst-case expected regret in \cref{eq:worst case exp regret finite} admits a dual formulation involving a single scalar variable only. Extending this idea, \cref{thm:infinite strong duality} presents a similar dual formulation for the infinite-horizon worst-case expected regret $R(\K,r)$, stated in \cref{eq:worst case exp regret infinite}, treating it as a single variable search problem. 

%\tk{redundant}
We introduce the following assumption on the nominal disturbances to guarantee that the nominal disturbances are weakly stationary.
\begin{assumption}\label{asmp:nominal} 
     A positive bi-infinite Toeplitz operator $\M_\circ$ exists such that $\Tr(\M_\circ) \< \infty$ and for any horizon $T\>0$, the nominal disturbance satisfies $ \E_{\Pr_\circ}[\wfin_{\circ} \wfin_{\circ}^\ast] \= [\M_\circ]_{T}$.
\end{assumption}
Note that, $\M_\circ = \I$ satisfies this assumption.

The proceeding theorem establishes strong duality for the worst-case expected regret, $R(\K,r)$ holds in the infinite horizon.
%\tk{BABAK, should I cite our L4DC paper for each former result? Do you think this is too much overlap? ICML says "papers that explicitly or implicitly reveal the authors’ identities will be rejected"; }
\begin{theorem}[\textbf{Strong duality of \eqref{eq:worst case exp regret infinite} in infinite horizon \fix{\citep[Thm. 5]{kargin2023wasserstein}}}] \label{thm:infinite strong duality}
Let $\K \in \causal$ be a causal and time-invariant policy. The infinite-horizon worst-case expected regret, $R(\K,r)$, suffered by $\K$ coincides with the optimal value of the following problem:
\begin{equation}\label{eq:dual_worst_case_regret} %\vspace{-2mm}
    \inf_{\gamma \geq 0 } \cl{  \gamma \Tr\br{ (\T_{\gamma}(\K)\- \I) \M_\circ}  \+ \gamma r^2 \!\mid \! \T_{\gamma}(\K)\!\psdg\! 0}
\end{equation}
where $\T_{\gamma}(\K) \defeq ( \I \- \gamma^{\-1}\RR(\K) )^{-1}$ is the $\gamma$-optimal transport map from the nominal disturbance. The worst-case disturbance $\w_\star$ is generated from the nominal disturbance as $\w_\star \= \T_{\gamma_\star}(\K) \,\w_\circ$ where the infimum is attained by a unique $\gamma_{\star} > \norm[\op]{\RR(\K)}$ which solves the following equation:
\begin{equation}\label{eq:worst_gamma} %\vspace{-2.5mm}
    \Tr\br{(\T_{\gamma_\star}(\K) - \I)^2 \M_\circ} = r^2.
\end{equation}  
\end{theorem}
\begin{proof}
    See \tk{appendix}
\end{proof}

Leveraging the dual problem in \cref{thm:infinite strong duality}, \DRO~ in \cref{prob:DR-RO} can be reformulated as follows:
\begin{equation}\label{eq:infinite DRRO reformulation}%\vspace{-1.5mm}
    \inf_{\substack{\gamma\geq 0 \\ \K \in \causal}} \{\gamma \Tr\br{ (\T_{\gamma}(\K)\- \I) \M_\circ}  \+ \gamma r^2 \mid \T_{\gamma}(\K)\!\psdg \!0 \},
\end{equation}
Observe that $\T_{\gamma}(\K)\!\psdg\! 0$ is equivalent to $\gamma\I \!\psdg \!\RR(\K)$, implying $\gamma \> \norm[\op]{\RR(\K)}$. Consequently, the optimal solution $\gamma_\star$ for any $r\>0$ must have a lower bound of ${\gamma}_{\RO} \defeq \inf_{\K\in\causal} \norm[\op]{\RR(\K)}$, signifying the worst-case regret of the $\RO$ controller.

As opposed to the $\gamma$-optimal problem formulated in \cref{prob:suboptimal_DR_RO}, the dependence of $\K$ on the objective function in \cref{eq:regularized suboptimal} is quadratic. If the min-max can be exchanged, then the infimum of $\Tr\pr{\RR(\K) \M}$ among all causal controllers can be done via the Wiener-Hopf technique \citep{kailath_linear_2000}.
\tk{pushable to the appendix}
 \begin{lemma}[{Wiener-Hopf Technique \citep{kailath_linear_2000}}]\label{lem:wiener}
    Let $\Delta^\ast \Delta = \I + \F^\ast \F$ be the canonical spectral factorization with causal $\Delta$, and $\Delta^\inv$. Given $\M\psdg 0$, consider the following minimization problem over causal controllers:
    \begin{equation}
        \inf_{\K \in\causal} \Tr(\RR(\K) \M ),
    \end{equation}
    where $\RR(\K) = \left(\K - \K_\circ \right)^{\ast}\Delta^{\ast}\Delta\left(\K - \K_\circ \right)$ The solution to this problem is given by 
    \begin{equation}
        \K = \Delta^\inv\cl{\Delta \K_\circ \L}_{\!+} \L^\inv,
        \label{eq: K from L}
    \end{equation}
    where $\L$ is the unique causal and causally invertible spectral factor of $\M$ such that $\M = \L \L^\ast$ and $\cl{ \cdot }_{\!+}$ denotes the causal part of an operator.
\end{lemma}

The \cref{thm:kkt} establishes the exchange of min-max in \cref{eq:regularized suboptimal} and using the Wiener-Hopf technique in \cref{lem:wiener}, provides the solution to the $\gamma$-optimal \DRO~ Problem~\ref{prob:suboptimal_DR_RO} through a saddle point.

\begin{problem}[\textbf{$\gamma$-optimal \DRO~control}] \label{prob:suboptimal_DR_RO}
For a fixed $\gamma >{\gamma}_{\RO}$, find a causal control policy, $\K_{\gamma,\star}$, that minimizes the $\gamma$-optimal objective function in \cref{eq:dual_worst_case_regret}, \ie %\vspace{-3mm}
\begin{equation}\label{eq:suboptimal objective K only}
       %\inf_{\K \in\causal } \Tr{ ( \I - \gamma^{\-1}\CC_{\K} )^{\-1}} \quad \textrm{s.t.} \quad \gamma \I \psdg \CC_{\K}.
    %\inf_{\K \in \causal} \cl{\gamma \Tr\br{ (\T_{\gamma}(\K)- \I) \M_\circ}  \mid \T_{\gamma}(\K)\!\psdg \!0 },
    \nu_{\gamma} \defeq \inf_{\K \in \causal} \gamma \Tr\br{ (\T_{\gamma}(\K)- \I) \M_\circ }\,\textrm{ s.t. }\, \T_{\gamma}(\K)\!\psdg \!0.
\end{equation}
\end{problem}

\begin{remark}\label{remark:limiting_r}
As $r\to\infty$, the optimal $\gamma_\star$ approaches the lower bound $\norm[\op]{\RR(\K)}$, the worst-case regret as in \cref{prob:regret_optimal}, and the optimal \DRO~controller recovers the regret-optimal ($\RO$) controller. Conversely, as $r\to 0$,  $\gamma_\star \to \infty$, leading the worst-case expected regret $R(\K_{\gamma,\star}, r)$ to be the expected regret under nominal disturbance, $\M_\circ$, and the optimal \DRO~controller recovers the $\Htwo$ controller when $\M_\circ = \I$. Adjusting $r$ facilitates the \DRO~controller to interpolate between the $\RO$ and $\Htwo$ controllers.

\end{remark}

\subsection{A Saddle Point Solution to $\gamma$-optimal \DRO~ \cref{prob:suboptimal_DR_RO} }

%For a given fixed $\gamma>0$, if we can solve \cref{eq:DR-RO_reformulation} to obtain a $\gamma$-optimal controller, $\K_{\gamma,\star}$, then the optimal \DRO~controller can be obtained by searching for the optimal $\gamma_\star$ using \cref{eq:worst_gamma}. Therefore, we restrict our attention to the $\gamma$-optimal problem described below.

%${\gamma}_{\RO}  \defeq \inf \cl{\gamma \geq 0 \mid  \inf_{\K \in \causal} \tr\br{ \T_{\gamma}(\K)\M_\circ}  < \infty }$
The current form of \cref{prob:suboptimal_DR_RO} presents a challenge due to the nonlinearity introduced by the map $\K \mapsto \T_{\gamma}(\K) = (\I - \gamma^{-1}\RR(\K))^{-1}$, which appears both in the objective function and as a constraint. By leveraging Fenchel duality for the inverse mapping $\mathcal{X}\mapsto \Tr(\mathcal{X}^{-1})$, we can achieve an equivalent reformulation of \cref{prob:suboptimal_DR_RO}, as detailed in \cref{lem:regularized suboptimal objective}. Before delving into \cref{lem:regularized suboptimal objective}, we introduce the Bures-Wasserstein ($\BW$) metric, which plays a central role in formulating the min-max version of the $\gamma$-optimal problem.

%In its present form, \cref{prob:suboptimal_DR_RO} is challenging since the $\K \mapsto \T_{\gamma}(\K) =( \I \- \gamma^{\-1}\RR(\K) )^{-1}$ is a nonlinear map appearing both in the objective function as well as a constraint $\T_{\gamma}(\K)$. Leveraging Fenchel duality for inverse mapping $\clf{X}\mapsto \Tr(\clf{X}^{-1})$, an equivalent reformulation of \cref{prob:suboptimal_DR_RO} is presented in \cref{lem:regularized suboptimal objective}. Before moving on with \cref{lem:regularized suboptimal objective}, we introduce the Bures-Wasserstein ($\BW$) metric which plays a central role in our regularized $\gamma$-optimal problem formulation.

\begin{lemma}[\textbf{A min-max version of the $\gamma$-optimal \DRO~control}]\label{lem:regularized suboptimal objective}
Let $\gamma>{\gamma}_{\RO}$ be fixed. The $\gamma$-optimal \DRO~control problem in \cref{eq:suboptimal objective K only} is equivalent to the following $\BW$-regularized min-max problem
\begin{equation}\label{eq:regularized suboptimal}
    \nu_\gamma = \inf_{\K \in \causal} \sup_{\M \psdg 0} \Tr(\RR(\K) \M) - \gamma \BW(\M,\, \M_\circ)^2
\end{equation}
\end{lemma}
\begin{proof}
    See \tk{appendix}
\end{proof}
