# Supplementary material for: Distributionally Robust Kalman Filtering over Finite and Infinite Horizon
Source: arXiv:2407.18837 source file (2024-07-26)
Supplement: Supplementary file 2 [file old_appendix_5_rational.tex]

\subsection{Obtaining State-Space Estimators from Rational $N(\ejw)$} \jh{This is the filtering version}
